# Supplementary material for: Accurate optical spectra through time-dependent density functional theory based on screening-dependent hybrid functionals
Source: arXiv:2002.02222 source file (2020-08-14)
Supplement: Supplementary file 1 [file supplemental.pdf]

# Accurate optical spectra through time-dependent density functional theory based on screening-dependent hybrid functionals

Alexey Tal,[1,*] Peitao Liu,[2] Georg Kresse,[2] and Alfredo Pasquarello[1]

[1] *Chaire de Simulation à l'Echelle Atomique (CSEA), Ecole Polytechnique Fédérale de Lausanne (EPFL), CH-1015 Lausanne, Switzerland*

[2] *University of Vienna, Faculty of Physics and Center for Computational Materials Science, Sensengasse 8, A-1090 Vienna, Austria*

## COMPUTATIONAL DETAILS

The calculations are performed within the projector augmented wave (PAW) formalism [1] implemented in VASP [2, 3]. The Si_GW, C_GW, Mg_sv_GW, Na_sv_GW, Ar_GW, Cl_GW, and O_GW_new PAW potentials are used in the calculations. The convergence parameters of the calculations are provided in Table I.

TABLE I. Convergence parameters of the calculations.

| | $E_{\text{cutoff}}^{\text{DFT}}$(eV) | k-points | $N_{\text{bands}}$ | $E_{\text{cutoff}}^{\text{GW}}$(eV) | $N_\omega$ |
|---|---|---|---|---|---|
| Diamond | 414 | $6\times6\times6$ | 128 | 276 | 100 |
| Si | 245 | $6\times6\times6$ | 256 | 164 | 100 |
| SiC | 414 | $6\times6\times6$ | 256 | 276 | 100 |
| NaCl | 373 | $6\times6\times6$ | 384 | 249 | 100 |
| Ar | 291 | $6\times6\times6$ | 256 | 194 | 100 |
| MgO | 434 | $6\times6\times6$ | 256 | 290 | 100 |

The spectra are obtained as averages over eight calculations based on $6 \times 6 \times 6$ **k**-point grids shifted off the $\Gamma$ point. The shifts correspond to the irreducible points of a $\Gamma$-point centered $4\times4\times4$ **k**-point grid. This approach effectively gives the sampling of the Brillouin zone with $(6\times4)\times(6\times4)\times(6\times4) \approx 24\times24\times24$ **k**-points. The parameters of the employed DDH functionals, which also define the model dielectric functions, are taken from Ref. [4].

TABLE II. DDH parameters from Ref. [4].

| | $\epsilon_\infty$ | $\mu$ (bohr$^{-1}$) | Space group | $a_0$(Å) |
|---|---|---|---|---|
| Diamond | 5.47 | 0.9 | $Fd\bar{3}m$ | 3.567 |
| Si | 11.35 | 0.65 | $Fd\bar{3}m$ | 5.430 |
| SiC | 6.38 | 0.77 | $F\bar{4}3m$ | 4.358 |
| NaCl | 2.38 | 0.69 | $Fm\bar{3}m$ | 5.595 |
| Ar | 1.76 | 0.74 | $Fm\bar{3}m$ | 5.26 |
| MgO | 3.08 | 0.8 | $Fm\bar{3}m$ | 4.207 |

The BSE-*GW* approach referred to in the main text is the following. The starting wave functions and energies correspond to the DDH ground state. This choice gives an accurate

description of the band structure and speeds up the convergence of the $GW$ calculation. For the quasi-particle calculations we used the partially self-consistent $GW$ method with a "nanoquanta" kernel [5–9] for the vertex corrections. In this approach, the eigenvalues are updated self-consistently, while the wave functions remain unchanged. Finally, the quasi-particle energies and the dielectric matrix obtained in the $GW$ calculation are used to construct and solve the BSE in the Tamm-Dancoff approximation.

In the TD-DDH calculation, the DDH ground-state wave functions and energies are used in the construction of the Casida equation. In this case, the same approximated dielectric function, given in Eq. (3) of the main text, is used for screening the exchange interaction in the hybrid functional calculation and for screening the electron-hole interaction in the Casida equation in the Tamm-Dancoff approximation.

## COMPARISON OF TIME-DEPENDENT HYBRID FUNCTIONAL APPROACHES

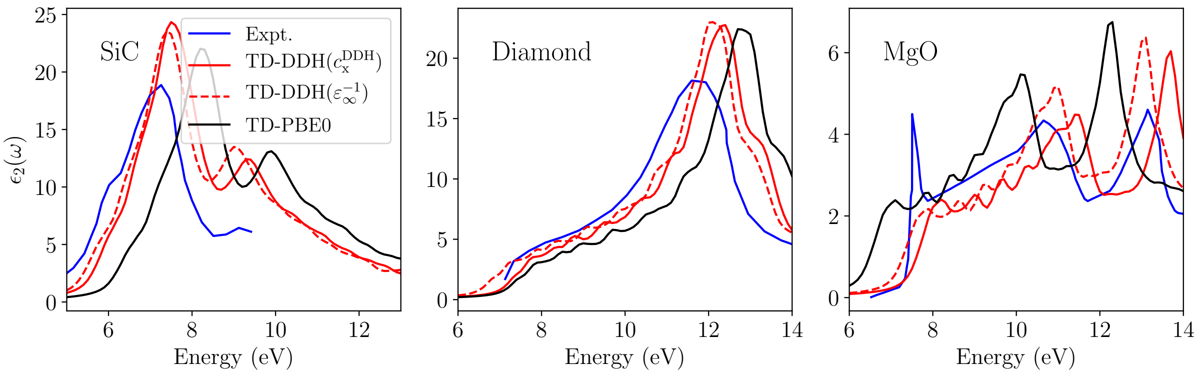


FIG. 1. Absorption spectra obtained with different TD-DFT approaches: the present TD-DDH($c_x^{\mathrm{DDH}}$) (red solid line) and TD-DDH($\varepsilon_\infty^{-1}$) (red dashed line). The comparison also includes the common TD-PBE0, in which the Fock mixing parameter is set to $\alpha = 0.25$ (black line). Experimental spectra are taken from [10] for diamond, from [11] for SiC, and from [12] for MgO (blue line).

In Fig. 1, TD-DDH spectra obtained with the model dielectric function in Eq. (3) of the main text and with a uniform screening ($\varepsilon_\infty$) are shown. Both methods yield spectra in good agreement with experiment. However, the TD-DDH($\varepsilon_\infty^{-1}$) approach underestimates the band gaps (Table III) and the agreement of the spectra with the experiment is the consequence

of a compensation effect resulting from the weaker electron-hole interaction. Moreover, TD-DDH($c_x^{\mathrm{DDH}}$) gives a better description of the dielectric function obtained with BSE-$GW$, which makes this scheme overall more reliable.

In order to assess the performance of TD-DDH compared to other hybrid functional approaches, we carried out calculations of the spectra with the TD-PBE0 scheme [13]. In the ground state calculations, this scheme uses 25% of Fock exchange and the exchange interaction in the calculation of the spectra is uniformly screened by the dielectric constant $\varepsilon_\infty$. The agreement with experiment is significantly worse for the spectra obtained with TD-PBE0 than for those achieved with the TD-DDH approaches. This discrepancy mostly originates from the inaccurate description of the single-particle energy levels (Table III).

TABLE III. Band gaps (in eV). The experimental values and the theoretical corrections resulting from the coupling to phonons are taken from Ref. [4].

| | TD-DDH($c_{\mathrm{x}}^{\mathrm{DDH}}$) | TD-DDH($\varepsilon_\infty^{-1}$) | TD-PBE0 | Expt. |
|---|---|---|---|---|
| SiC | 2.49 | 2.36 | 2.97 | 2.53 |
| C | 5.67 | 5.57 | 6.07 | 5.85 |
| MgO | 8.41 | 8.04 | 7.28 | 8.36 |

## QUASI-PARTICLE SELF-CONSISTENT QS$GW$ CALCULATIONS

To examine the effect of updating self-consistently the wave functions, we here perform additional fully self-consistent quasi-particle QS$GW$ [14] calculations including "nanoquanta" vertex corrections [9] for MgO, NaCl, and C. In Fig. 2, the calculated absorption spectra are compared with the results obtained with the methods discussed in the main text. Here, the calculations are performed with a lighter $16\times16\times16$ $\mathbf{k}$-point grid. The effect of updating the wave functions in the self-consistent QS$GW$ scheme does not lead to significant differences.

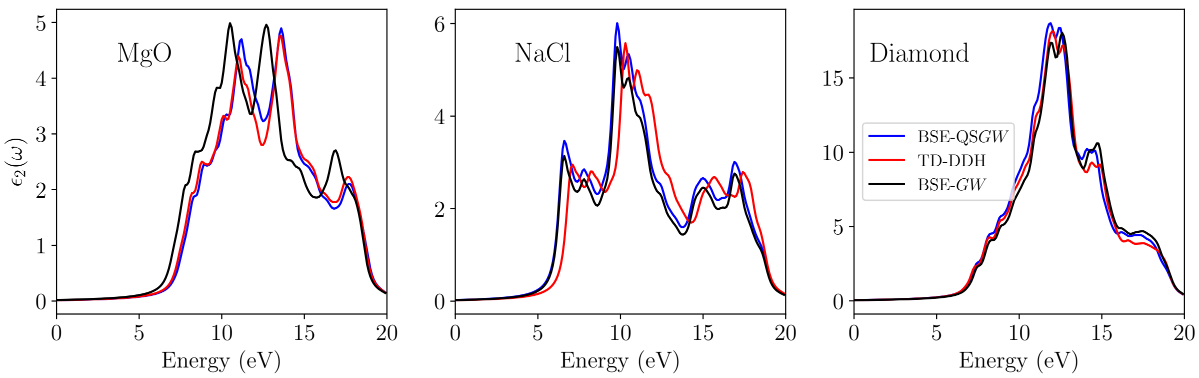


FIG. 2. Comparison of the spectra calculated with fully self-consistent BSE-QS$GW$, BSE-$GW$ and TD-DDH.

---

* alexey.tal@epfl.ch, alyxthal@gmail.com

[1] P. E. Blöchl, Projector augmented-wave method, Phys. Rev. B **50**, 17953 (1994).

[2] G. Kresse and J. Hafner, Ab initio molecular dynamics for liquid metals, Phys. Rev. B **47**, 558–561 (1993).

[3] G. Kresse and J. Furthmüller, Efficient iterative schemes for ab initio total-energy calculations using a plane-wave basis set, Phys. Rev. B **54**, 11169 (1996).

[4] W. Chen, G. Miceli, G. M. Rignanese, and A. Pasquarello, Nonempirical dielectric-dependent hybrid functional with range separation for semiconductors and insulators, Phys. Rev. Mater. **2**, 073803 (2018).

[5] L. Reining, V. Olevano, A. Rubio, G. Onida, A. Rubio, and G. Onida, Excitonic Effects in Solids Described by Time-Dependent Density-Functional Theory, Phys. Rev. Lett. **88**, 4 (2002).

[6] A. Marini, R. Del Sole, A. Rubio, R. D. Sole, and A. Rubio, Bound excitons in time-dependent density-functional theory: Optical and energy-loss spectra, Phys. Rev. Lett. **91**, 256402 (2003).

[7] F. Sottile, V. Olevano, and L. Reining, Parameter-free calculation of response functions in time-dependent density-functional theory, Phys. Rev. Lett. **91**, 056402 (2003).

[8] F. Bruneval, F. Sottile, V. Olevano, R. Del Sole, and L. Reining, Many-Body Perturbation Theory Using the Density-Functional Concept: Beyond the $GW$ Approximation, Phys. Rev. Lett. **94**, 186402 (2005).

[9] M. Shishkin, M. Marsman, and G. Kresse, Accurate quasiparticle spectra from self-consistent *GW* calculations with vertex corrections, Phys. Rev. Lett. **99**, 246403 (2007).

[10] E. D. Palik, *Handb. Opt. Constants Solids*, Vol. 1 (Academic Press, 2012) pp. 1–804.

[11] S. Logothetidis and J. Petalas, Dielectric function and reflectivity of 3C-silicon carbide and the component perpendicular to the c axis of 6H-silicon carbide in the energy region 1.5-9.5 eV, J. Appl. Phys. **80**, 1768–1772 (1996).

[12] M. L. Bortz, R. H. French, D. J. Jones, R. V. Kasowski, and F. S. Ohuchi, *Phys. Scr.*, Tech. Rep. (1990).

[13] Z.-h. Yang, F. Sottile, and C. A. Ullrich, Simple screened exact-exchange approach for excitonic properties in solids, Phys. Rev. B **92**, 035202 (2015).

[14] M. van Schilfgaarde, T. Kotani, and S. Faleev, Quasiparticle Self-Consistent *GW* Theory, Phys. Rev. Lett. **96**, 226402 (2006).

[15] C. Adamo and V. Barone, Toward reliable density functional methods without adjustable parameters: The PBE0 model, The Journal of Chemical Physics **110**, 6158 (1999).

[16] J. P. Perdew, M. Ernzerhof, and K. Burke, Rationale for mixing exact exchange with density functional approximations, The Journal of Chemical Physics **105**, 9982 (1996).

[17] F. Santoro and D. Jacquemin, Going beyond the vertical approximation with time-dependent density functional theory, **6**, 460 (2016).
